# Supplementary material for: Magnetic circular dichroism within the Algebraic Diagrammatic Construction scheme of the polarisation propagator up to third order
Source: arXiv:2203.11344 source file (2022-03-21)
Supplement: Supplementary file 1 [file SI_v2.pdf]

**Magnetic circular dichroism within the Algebraic Diagrammatic Construction scheme of the polarisation propagator up to third order. Supplementary Information.**

Daniil A. Fedotov,<sup>1</sup> Mikael Scott,<sup>2</sup> Maximilian Scheurer,<sup>2</sup> Dirk R. Rehn,<sup>2</sup> Andreas Dreuw,<sup>2, a)</sup> and Sonia Coriani<sup>1, b)</sup>

<sup>1)</sup>*DTU Chemistry, Technical University of Denmark, Kemitorvet, Building 207, DK-2800 Kongens Lyngby, Denmark*

<sup>2)</sup>*University of Heidelberg Im Neuenheimer Feld 205A 69120, Heidelberg, Germany*

---

<sup>a)</sup>Electronic mail: dreuw@uni-heidelberg.de

<sup>b)</sup>Electronic mail: soco@kemi.dtu.dk

## 1. MCD AND OPA SPECTRA

### 1.1. Uracil, 2-thiouracil and 4-thiouracil

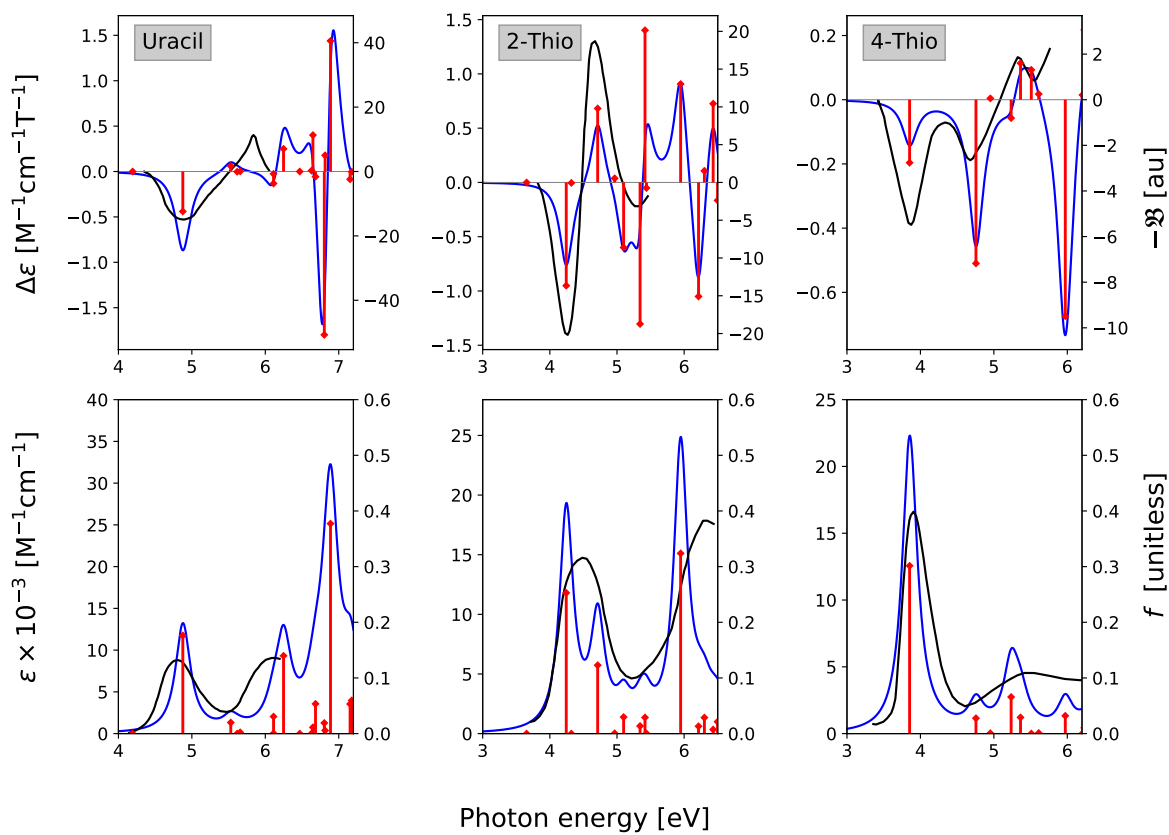

Figure S1. Uracil, 2-thiouracil, 4-thiouracil. MCD (upper panels) and OPA spectra (lower panels) at ADC(2)-x level. The computed spectra were shifted to align with the lowest energy experimental band, by  $-0.3$  eV,  $-0.5$  eV and  $-0.65$  eV for uracil, 2-thiouracil and 4-thiouracil, respectively. Experimental spectra, recorded in water, digitized from Refs.1 and 2 are shown as black lines.

Table S1: Uracil. ADC(2)/aug-cc-pVDZ results for excitation wavelengths  $\lambda_n$  (nm), excitation energies  $E_n$  (Hartree), oscillator strengths  $f$  and MCD  $-\mathcal{B}$  terms (atomic units) at planar geometry (MP2/cc-pVTZ optimized).

| State $n$ | $\lambda_n$ | $E_n$ | $f$   | $-\mathcal{B}$ | Symm. |
|-----------|-------------|-------|-------|----------------|-------|
| 1         | 266.452     | 0.171 | 0.000 | -0.002         | 1A''  |
| 2         | 234.139     | 0.195 | 0.209 | -12.872        | 1A'   |
| 3         | 212.120     | 0.215 | 0.003 | 0.049          | 2A''  |
| 4         | 207.767     | 0.219 | 0.000 | -0.041         | 3A''  |
| 5         | 201.163     | 0.227 | 0.013 | 2.912          | 2A'   |
| 6         | 199.141     | 0.229 | 0.058 | 0.260          | 3A'   |
| 7         | 190.164     | 0.240 | 0.001 | -0.881         | 4A''  |
| 8         | 185.594     | 0.246 | 0.105 | -0.699         | 4A'   |
| 9         | 182.765     | 0.249 | 0.012 | 19.044         | 5A''  |
| 10        | 182.472     | 0.250 | 0.094 | -0.637         | 5A'   |
| 11        | 181.745     | 0.251 | 0.004 | -9.323         | 6A''  |
| 12        | 180.592     | 0.252 | 0.000 | -0.006         | 7A''  |
| 13        | 179.454     | 0.254 | 0.057 | -19.467        | 6A'   |
| 14        | 176.192     | 0.259 | 0.003 | 0.216          | 8A''  |
| 15        | 172.785     | 0.264 | 0.140 | 14.865         | 7A'   |
| 16        | 170.841     | 0.267 | 0.009 | 0.753          | 8A'   |
| 17        | 167.697     | 0.272 | 0.354 | 12.054         | 9A'   |
| 18        | 166.533     | 0.274 | 0.001 | 0.283          | 9A''  |

Table S2: Uracil. ADC(2)-x/aug-cc-pVDZ results for excitation wavelengths  $\lambda_n$  (nm), excitation energies  $E_n$  (Hartree), oscillator strengths  $f$  and MCD  $-\mathcal{B}$  terms (atomic units) at planar geometry (MP2/cc-pVTZ optimized).

| State $n$ | $\lambda_n$ | $E_n$ | $f$   | $-\mathcal{B}$ | Symm. |
|-----------|-------------|-------|-------|----------------|-------|
| 1         | 318.402     | 0.143 | 0     | 0.000          | 1A''  |
| 2         | 270.888     | 0.168 | 0.176 | -12.416        | 1A'   |
| 3         | 237.062     | 0.192 | 0.020 | 1.693          | 2A'   |
| 4         | 233.180     | 0.195 | 0.000 | -0.064         | 2A''  |
| 5         | 231.404     | 0.197 | 0.002 | 0.048          | 3A''  |
| 6         | 213.312     | 0.214 | 0.031 | -0.736         | 3A'   |
| 7         | 213.312     | 0.214 | 0.000 | -3.721         | 4A''  |
| 8         | 208.433     | 0.219 | 0.140 | 7.045          | 4A'   |
| 9         | 200.985     | 0.227 | 0.000 | -0.003         | 5A''  |
| 10        | 195.887     | 0.233 | 0.000 | 0.269          | 6A''  |
| 11        | 195.299     | 0.233 | 0.011 | 11.307         | 7A''  |
| 12        | 194.217     | 0.235 | 0.054 | -1.616         | 5A'   |
| 13        | 190.642     | 0.239 | 0.019 | -50.735        | 6A'   |
| 14        | 190.323     | 0.239 | 0.006 | 5.025          | 8A''  |
| 15        | 188.201     | 0.242 | 0.377 | 40.566         | 7A'   |
| 16        | 180.879     | 0.252 | 0.053 | -2.413         | 8A'   |
| 17        | 180.306     | 0.253 | 0.060 | -0.074         | 9A'   |

Table S3: Uracil. ADC(3)/aug-cc-pVDZ results for excitation wavelengths  $\lambda_n$  (nm), excitation energies  $E_n$  (Hartree), oscillator strengths  $f$  and MCD  $-\mathcal{B}$  terms (atomic units) at planar geometry (MP2/cc-pVTZ optimized).

| State $n$ | $\lambda_n$ | $E_n$ | $f$   | $-\mathcal{B}$ | Symm. |
|-----------|-------------|-------|-------|----------------|-------|
| 1         | 233.180     | 0.195 | 0.000 | -0.061         | 1A''  |
| 2         | 231.875     | 0.197 | 0.214 | -11.851        | 1A'   |
| 3         | 211.039     | 0.216 | 0.004 | 0.131          | 2A''  |
| 4         | 189.295     | 0.241 | 0.036 | 6.182          | 2A'   |
| 5         | 182.472     | 0.250 | 0.000 | 9.643          | 3A''  |
| 6         | 182.399     | 0.250 | 0.185 | -9.958         | 3A'   |
| 7         | 181.383     | 0.251 | 0.017 | -4.114         | 4A''  |
| 8         | 179.950     | 0.253 | 0.003 | 3.391          | 5A''  |
| 9         | 169.381     | 0.269 | 0.005 | 1.491          | 4A'   |
| 10        | 166.229     | 0.274 | 0.001 | -0.863         | 6A''  |
| 11        | 161.172     | 0.283 | 0.198 | 1.463          | 5A'   |

Table S4: Uracil. RICC2/aug-cc-pVDZ results for excitation wavelengths  $\lambda_n$  (nm), excitation energies  $E_n$  (Hartree), oscillator strengths  $f$  and MCD  $-\mathcal{B}$  terms (atomic units) at planar geometry (MP2/cc-pVTZ optimized).

| State $n$ | $\lambda_n$ | $E_n$ | $f$   | $-\mathcal{B}$ | Symm. |
|-----------|-------------|-------|-------|----------------|-------|
| 1         | 253.106     | 0.180 | 0.000 | -0.003         | 1A''  |
| 2         | 229.815     | 0.198 | 0.181 | -12.113        | 1A'   |
| 3         | 212.329     | 0.215 | 0.003 | -0.063         | 2A''  |
| 4         | 200.264     | 0.228 | 0.000 | 0.010          | 3A''  |
| 5         | 197.457     | 0.231 | 0.001 | 0.002          | 2A'   |
| 6         | 195.179     | 0.233 | 0.072 | -0.233         | 3A'   |
| 7         | 186.646     | 0.244 | 0.001 | -1.118         | 4A''  |
| 8         | 183.985     | 0.248 | 0.118 | -4.609         | 4A'   |
| 9         | 183.064     | 0.249 | 0.016 | 14.514         | 5A''  |
| 10        | 182.549     | 0.250 | 0.001 | 3.530          | 6A''  |
| 11        | 180.317     | 0.253 | 0.075 | -1.911         | 5A'   |
| 12        | 176.533     | 0.258 | 0.052 | -18.848        | 6A'   |
| 13        | 175.303     | 0.260 | 0.001 | 2.764          | 7A''  |
| 14        | 175.132     | 0.260 | 0.000 | -0.046         | 8A''  |
| 15        | 171.544     | 0.266 | 0.032 | 6.716          | 7A'   |
| 16        | 169.530     | 0.269 | 0.028 | 0.853          | 8A'   |
| 17        | 164.839     | 0.276 | 0.389 | 15.796         | 9A'   |
| 18        | 164.464     | 0.277 | 0.001 | 3.721          | 9A''  |
| 19        | 163.133     | 0.279 | 0.001 | -0.279         | 10A'' |

Table S5: Uracil + 4· H<sub>2</sub>O. ADC(2)/aug-cc-pVDZ results for excitation wavelengths  $\lambda_n$  (nm), excitation energies  $E_n$  (Hartree), oscillator strengths  $f$  and MCD  $-\mathcal{B}$  terms (atomic units) at the PCM-B3LYP/cc-pVTZ optimized structure, taken from Ref. 3.

| State $n$ | $\lambda_n$ | $E_n$ | $-\mathcal{B}$ |
|-----------|-------------|-------|----------------|
| 1         | 253.411     | 0.180 | 0.031          |
| 2         | 240.694     | 0.189 | -15.826        |
| 3         | 204.687     | 0.223 | 1.071          |
| 4         | 202.145     | 0.225 | 9.833          |
| 5         | 201.430     | 0.226 | -4.428         |
| 6         | 193.722     | 0.235 | -6.385         |
| 7         | 190.881     | 0.239 | 0.113          |

Table S6: 2-thiouracil. ADC(2)/aug-cc-pVDZ results for excitation wavelengths  $\lambda_n$  (nm), excitation energies  $E_n$  (Hartree), oscillator strengths  $f$  and MCD  $-\mathcal{B}$  terms (atomic units) at planar geometry (RI-MP2/cc-pVTZ optimized).

| State $n$ | $\lambda_n$ | $E_n$ | $f$   | $-\mathcal{B}$ | Symm. |
|-----------|-------------|-------|-------|----------------|-------|
| 1         | 321.321     | 0.142 | 0     | 0.000          | 1A''  |
| 2         | 277.318     | 0.164 | 0.379 | -12.882        | 1A'   |
| 3         | 270.085     | 0.169 | 0.000 | -0.126         | 2A''  |
| 4         | 248.437     | 0.183 | 0.082 | 10.768         | 2A'   |
| 5         | 233.061     | 0.196 | 0.002 | 0.183          | 3A''  |
| 6         | 229.538     | 0.199 | 0.016 | -21.173        | 4A''  |
| 7         | 226.683     | 0.201 | 0.033 | 17.314         | 3A'   |
| 8         | 224.782     | 0.203 | 0.038 | -5.620         | 4A'   |
| 9         | 222.044     | 0.205 | 0.000 | 0.339          | 5A''  |
| 10        | 199.228     | 0.229 | 0.331 | 73.693         | 5A'   |
| 11        | 198.706     | 0.229 | 0.014 | -67.984        | 6A''  |
| 12        | 195.049     | 0.234 | 0.102 | -22.376        | 6A'   |
| 13        | 192.738     | 0.236 | 0.024 | 35.279         | 7A'   |
| 14        | 192.169     | 0.237 | 0.011 | -6.578         | 7A''  |
| 15        | 185.217     | 0.246 | 0.000 | -1.151         | 8A''  |
| 16        | 183.354     | 0.249 | 0.031 | -5.644         | 8A'   |
| 17        | 179.737     | 0.254 | 0.004 | 2.917          | 9A'   |
| 18        | 178.610     | 0.255 | 0.016 | 13.051         | 9A''  |
| 19        | 178.051     | 0.256 | 0.044 | -12.781        | 10A'  |

Table S7: 2-thiouracil. ADC(2)-x/aug-cc-pVDZ results for excitation wavelengths  $\lambda_n$  (nm), excitation energies  $E_n$  (Hartree), oscillator strengths  $f$  and MCD  $-\mathcal{B}$  terms (atomic units) at planar geometry (RI-MP2/cc-pVTZ optimized).

| State $n$ | $\lambda_n$ | $E_n$ | $f$   | $-\mathcal{B}$ | Symm. |
|-----------|-------------|-------|-------|----------------|-------|
| 1         | 393.127     | 0.116 | 0     | -0.006         | 1A''  |
| 2         | 331.129     | 0.138 | 0.253 | -13.665        | 1A'   |
| 3         | 324.525     | 0.140 | 0.000 | -0.062         | 2A''  |
| 4         | 294.337     | 0.155 | 0.123 | 9.789          | 2A'   |
| 5         | 277.656     | 0.164 | 0.001 | 0.548          | 3A''  |
| 6         | 269.606     | 0.169 | 0.030 | -8.614         | 3A'   |
| 7         | 255.974     | 0.178 | 0.014 | -18.737        | 4A''  |
| 8         | 252.149     | 0.181 | 0.029 | 20.143         | 4A'   |
| 9         | 251.038     | 0.182 | 0.000 | -0.733         | 5A''  |
| 10        | 227.589     | 0.200 | 0.324 | 13.022         | 5A'   |
| 11        | 216.968     | 0.210 | 0.013 | -15.098        | 6A''  |
| 12        | 213.712     | 0.213 | 0.029 | 1.538          | 6A'   |
| 13        | 209.006     | 0.218 | 0.007 | 10.427         | 7A''  |
| 14        | 206.730     | 0.220 | 0.021 | -2.379         | 7A'   |
| 15        | 202.774     | 0.225 | 0.000 | 0.295          | 8A''  |
| 16        | 198.188     | 0.230 | 0.025 | -7.851         | 8A'   |

Table S8: 2-thiouracil. ADC(3)/aug-cc-pVDZ results for excitation wavelengths  $\lambda_n$  (nm), excitation energies  $E_n$  (Hartree), oscillator strengths  $f$  and MCD  $-\mathcal{B}$  terms (atomic units) at planar geometry (RI-MP2/cc-pVTZ optimized).

| State $n$ | $\lambda_n$ | $E_n$ | $f$   | $-\mathcal{B}$ | Symm. |
|-----------|-------------|-------|-------|----------------|-------|
| 1         | 298.190     | 0.153 | 0.000 | -0.002         | 1A''  |
| 2         | 267.862     | 0.170 | 0.293 | -21.345        | 1A'   |
| 3         | 245.360     | 0.186 | 0.157 | 13.665         | 2A'   |
| 4         | 237.929     | 0.192 | 0.000 | 0.290          | 2A''  |
| 5         | 232.466     | 0.196 | 0.018 | 0.321          | 3A''  |
| 6         | 216.762     | 0.210 | 0.057 | 8.240          | 3A'   |
| 7         | 215.430     | 0.212 | 0.039 | -13.894        | 4A'   |
| 8         | 212.714     | 0.214 | 0.001 | 0.794          | 4A''  |
| 9         | 200.720     | 0.227 | 0.015 | -1.214         | 5A''  |
| 10        | 193.393     | 0.236 | 0.008 | 123.931        | 6A''  |
| 11        | 193.311     | 0.236 | 0.269 | -112.206       | 5A'   |
| 12        | 188.278     | 0.242 | 0.071 | 4.161          | 6A'   |
| 13        | 182.472     | 0.250 | 0.016 | -13.861        | 7A''  |
| 14        | 181.023     | 0.252 | 0.012 | 4.832          | 7A'   |
| 15        | 180.092     | 0.253 | 0.005 | 8.042          | 8A''  |
| 16        | 179.031     | 0.255 | 0.024 | -4.565         | 8A'   |
| 17        | 176.739     | 0.258 | 0.002 | -0.118         | 9A''  |

Table S9: 2-thiouracil. RICC2/aug-cc-pVDZ results for excitation wavelengths  $\lambda_n$  (nm), excitation energies  $E_n$  (Hartree), oscillator strengths  $f$  and MCD  $-\mathcal{B}$  terms (atomic units) at planar geometry (RI-MP2/cc-pVTZ optimized).

| State $n$ | $\lambda_n$ | $E_n$ | $f$   | $-\mathcal{B}$ | Symm. |
|-----------|-------------|-------|-------|----------------|-------|
| 1         | 307.437     | 0.148 | 0.000 | 0.001          | 1A''  |
| 2         | 268.001     | 0.170 | 0.325 | -16.375        | 1A'   |
| 3         | 258.410     | 0.176 | 0.000 | -0.072         | 2A''  |
| 4         | 243.765     | 0.187 | 0.139 | 8.612          | 2A'   |
| 5         | 229.790     | 0.198 | 0.015 | -6.968         | 3A''  |
| 6         | 229.281     | 0.199 | 0.002 | -2.562         | 4A''  |
| 7         | 223.981     | 0.203 | 0.044 | 16.027         | 3A'   |
| 8         | 220.698     | 0.206 | 0.024 | -10.013        | 4A'   |
| 9         | 214.502     | 0.212 | 0.000 | 0.118          | 5A''  |
| 10        | 198.950     | 0.229 | 0.013 | -0.761         | 6A''  |
| 11        | 195.600     | 0.233 | 0.095 | 13.777         | 5A'   |
| 12        | 192.702     | 0.236 | 0.009 | -215.580       | 7A''  |
| 13        | 192.630     | 0.237 | 0.289 | 186.486        | 6A'   |
| 14        | 190.282     | 0.239 | 0.044 | 26.418         | 7A'   |
| 15        | 185.238     | 0.246 | 0.000 | -0.609         | 8A''  |
| 16        | 182.226     | 0.250 | 0.039 | -8.662         | 8A'   |
| 17        | 178.929     | 0.255 | 0.016 | 94.045         | 9A''  |
| 18        | 178.810     | 0.255 | 0.005 | -86.494        | 9A'   |
| 19        | 178.105     | 0.256 | 0.045 | -4.240         | 10A'  |

Figure S2. 2-thiouracil. OPA and MCD spectra and ADC(2) NTOs relative to the two states involved in the first bisignate band.

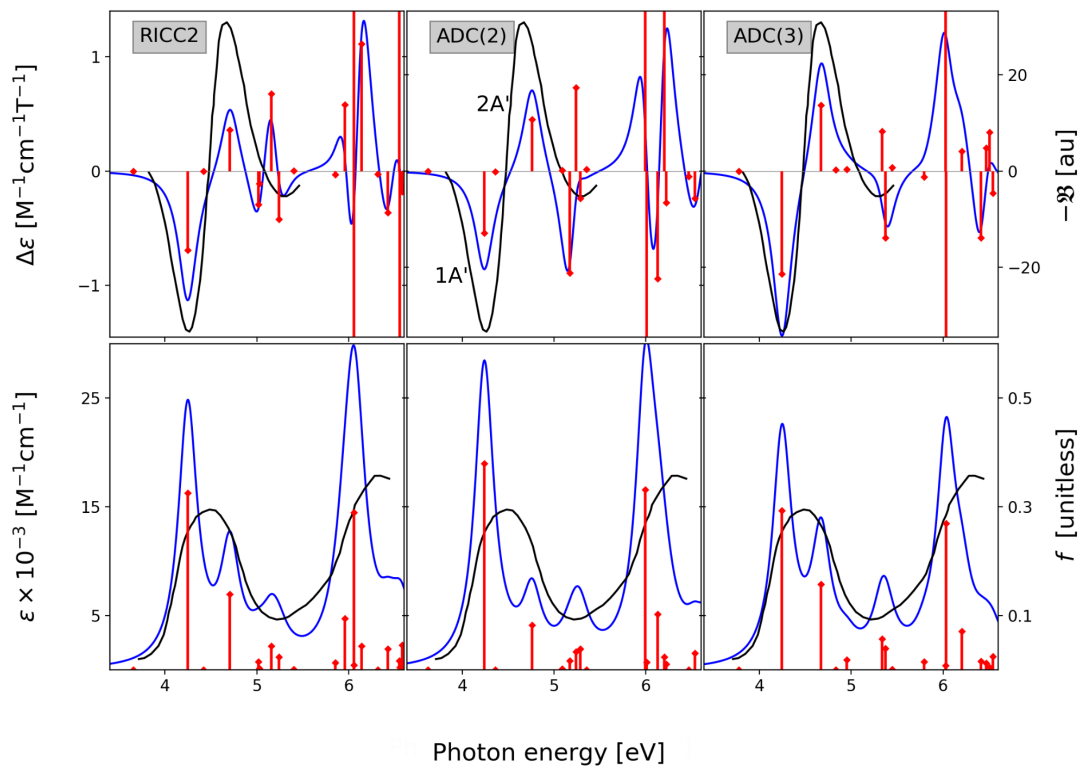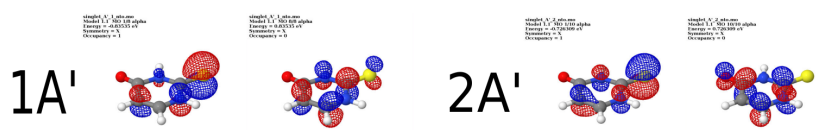

Table S10: 4-thiouracil. ADC(2)/aug-cc-pVDZ results for excitation wavelengths  $\lambda_n$  (nm), excitation energies  $E_n$  (Hartree), oscillator strengths  $f$  and MCD  $-\mathcal{B}$  terms (atomic units) at planar geometry (B3LYP/cc-pVTZ optimized).

| State $n$ | $\lambda_n$ | $E_n$ | $f$   | $-\mathcal{B}$ | Symm. |
|-----------|-------------|-------|-------|----------------|-------|
| 1         | 431.471     | 0.106 | 0.000 | 0.027          | 1A''  |
| 2         | 306.411     | 0.149 | 0.448 | -4.534         | 1A'   |
| 3         | 252.149     | 0.181 | 0.007 | -1.503         | 2A'   |
| 4         | 235.591     | 0.193 | 0.001 | 0.203          | 2A''  |
| 5         | 231.639     | 0.197 | 0.036 | -3.264         | 3A'   |
| 6         | 227.589     | 0.200 | 0.000 | 0.763          | 3A''  |
| 7         | 223.899     | 0.204 | 0.048 | 0.291          | 4A'   |
| 8         | 222.152     | 0.205 | 0.002 | 2.588          | 4A''  |
| 9         | 208.910     | 0.218 | 0.044 | -11.822        | 5A'   |
| 10        | 202.324     | 0.225 | 0.013 | 5.149          | 5A''  |
| 11        | 199.228     | 0.229 | 0.000 | -0.044         | 6A''  |
| 12        | 197.586     | 0.231 | 0.008 | -0.825         | 6A'   |
| 13        | 193.639     | 0.235 | 0.004 | -1.090         | 7A''  |
| 14        | 189.689     | 0.240 | 0.001 | -1.896         | 8A''  |
| 15        | 187.890     | 0.243 | 0.043 | 11.522         | 7A'   |
| 16        | 185.443     | 0.246 | 0.353 | 1.941          | 8A'   |
| 17        | 184.991     | 0.246 | 0.000 | 2.591          | 9A''  |
| 18        | 182.326     | 0.250 | 0.059 | -1.975         | 9A'   |
| 19        | 180.021     | 0.253 | 0.080 | -7.314         | 10A'  |

Table S11: 4-thiouracil. ADC(2)-x/aug-cc-pVDZ results for excitation wavelengths  $\lambda_n$  (nm), excitation energies  $E_n$  (Hartree), oscillator strengths  $f$  and MCD  $-\mathcal{B}$  terms (atomic units) at planar geometry (B3LYP/cc-pVTZ optimized).

| State $n$ | $\lambda_n/\text{nm}$ | $E_n/\text{Ha}$ | $f$   | $-\mathcal{B}/\text{a.u.}$ | Symm. |
|-----------|-----------------------|-----------------|-------|----------------------------|-------|
| 1         | 598.730               | 0.076           | 0.000 | 0.024                      | 1A''  |
| 2         | 387.114               | 0.118           | 0.302 | -2.762                     | 1A'   |
| 3         | 301.944               | 0.151           | 0.028 | -7.176                     | 2A'   |
| 4         | 288.193               | 0.158           | 0.001 | 0.058                      | 2A''  |
| 5         | 270.406               | 0.169           | 0.066 | -0.806                     | 3A'   |
| 6         | 263.068               | 0.173           | 0.029 | 1.602                      | 4A'   |
| 7         | 255.114               | 0.179           | 0.000 | 1.311                      | 3A''  |
| 8         | 249.936               | 0.182           | 0.001 | 0.248                      | 4A''  |
| 9         | 232.942               | 0.196           | 0.032 | -9.490                     | 5A'   |
| 10        | 223.131               | 0.204           | 0.000 | 0.208                      | 5A''  |
| 11        | 222.152               | 0.205           | 0.010 | 3.061                      | 6A''  |
| 12        | 219.055               | 0.208           | 0.006 | -1.437                     | 6A'   |

Table S12: 4-thiouracil. ADC(3)/aug-cc-pVDZ results for excitation wavelengths  $\lambda_n$  (nm), excitation energies  $E_n$  (Hartree), oscillator strengths  $f$  and MCD  $-\mathcal{B}$  terms (atomic units) at planar geometry (B3LYP/cc-pVTZ optimized).

| State $n$ | $\lambda_n$ | $E_n$ | $f$   | $-\mathcal{B}$ | Symm. |
|-----------|-------------|-------|-------|----------------|-------|
| 1         | 403.573     | 0.113 | 0.000 | 0.015          | 1A''  |
| 2         | 308.904     | 0.148 | 0.376 | -3.497         | 1A'   |
| 3         | 241.715     | 0.189 | 0.017 | -5.114         | 2A'   |
| 4         | 231.875     | 0.197 | 0.000 | -1.151         | 2A''  |
| 5         | 228.502     | 0.199 | 0.078 | -0.830         | 3A'   |
| 6         | 217.486     | 0.210 | 0.002 | 4.155          | 3A''  |
| 7         | 216.453     | 0.211 | 0.044 | -5.350         | 4A'   |
| 8         | 205.983     | 0.221 | 0.012 | -0.849         | 4A''  |
| 9         | 197.415     | 0.231 | 0.034 | -55.456        | 5A'   |
| 10        | 197.329     | 0.231 | 0.004 | 57.700         | 5A''  |
| 11        | 188.278     | 0.242 | 0.008 | -5.284         | 6A'   |

Table S13: 4-thiouracil. RICC2/aug-cc-pVDZ results for excitation wavelengths  $\lambda_n$  (nm), excitation energies  $E_n$  (Hartree), oscillator strengths  $f$  and MCD  $-\mathcal{B}$  terms (atomic units) at planar geometry (B3LYP/cc-pVTZ optimized).

| State $n$ | $\lambda_n$ | $E_n$ | $f$   | $-\mathcal{B}$ | Symm. |
|-----------|-------------|-------|-------|----------------|-------|
| 1         | 402.531     | 0.113 | 0.000 | 0.023          | 1A''  |
| 2         | 289.813     | 0.157 | 0.429 | -7.069         | 1A'   |
| 3         | 245.611     | 0.186 | 0.008 | -0.461         | 2A'   |
| 4         | 231.681     | 0.197 | 0.001 | 0.876          | 2A''  |
| 5         | 229.498     | 0.199 | 0.042 | -5.652         | 3A'   |
| 6         | 227.742     | 0.200 | 0.000 | 2.145          | 3A''  |
| 7         | 221.790     | 0.205 | 0.052 | 3.477          | 4A'   |
| 8         | 215.953     | 0.211 | 0.002 | 0.581          | 4A''  |
| 9         | 207.326     | 0.220 | 0.048 | -13.678        | 5A'   |
| 10        | 202.404     | 0.225 | 0.010 | 6.915          | 5A''  |
| 11        | 196.186     | 0.232 | 0.009 | 1.189          | 6A'   |
| 12        | 193.992     | 0.235 | 0.004 | -2.828         | 6A''  |
| 13        | 190.830     | 0.239 | 0.000 | 4.086          | 7A''  |
| 14        | 189.352     | 0.241 | 0.002 | -1.486         | 8A''  |
| 15        | 186.379     | 0.244 | 0.017 | 6.514          | 7A'   |
| 16        | 183.640     | 0.248 | 0.001 | -0.974         | 9A''  |
| 17        | 182.059     | 0.250 | 0.164 | 3.908          | 8A'   |
| 18        | 181.026     | 0.252 | 0.045 | 3.553          | 9A'   |
| 19        | 179.167     | 0.254 | 0.294 | 2.854          | 10A'  |

## 1.2. Purine and Hypoxanthine

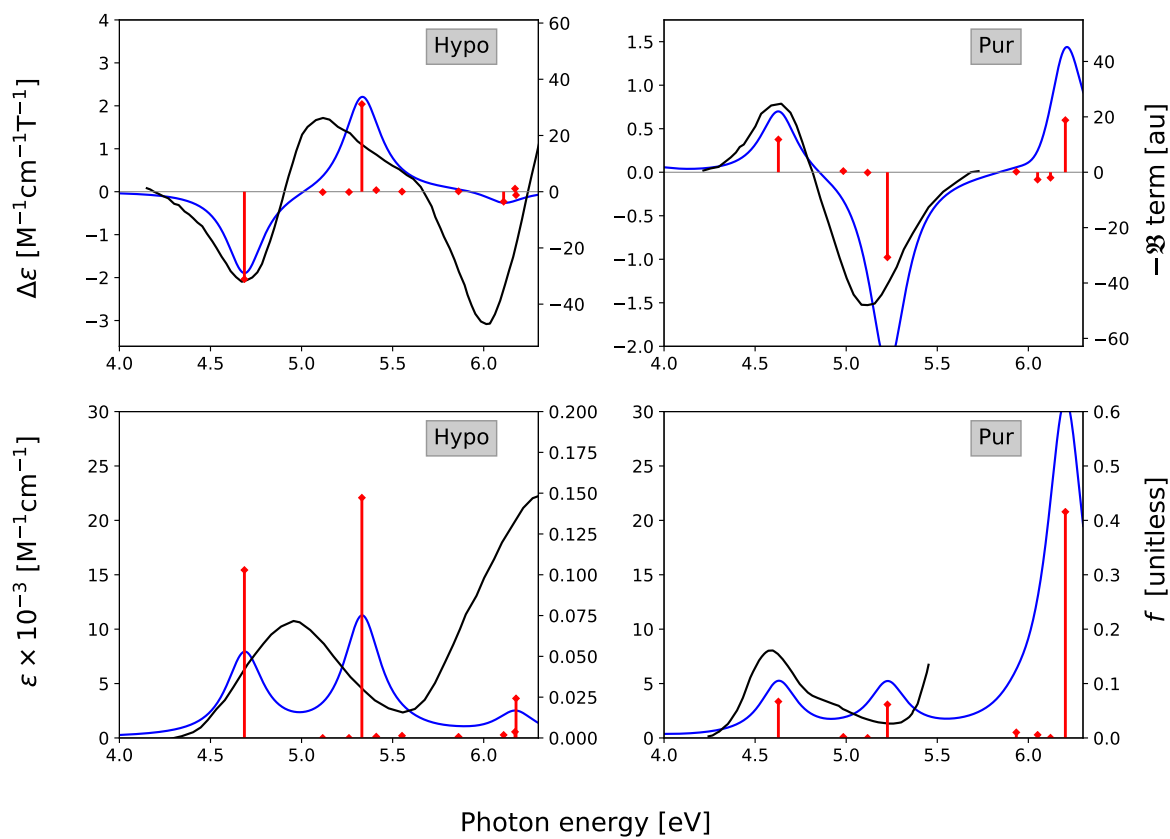

Figure S3. Purine and Hypoxanthine. MCD (upper panels) and OPA spectra (lower panels) at ADC(2)-x level. Experimental spectra, digitized from Refs. 4 and 5, are shown in black.

Table S14: Purine. ADC(2)/aug-cc-pVDZ results for excitation wavelengths  $\lambda_n$  (nm), excitation energies  $E_n$  (Hartree), oscillator strengths  $f$  and MCD  $-\mathcal{B}$  terms (atomic units) at planar geometry (MP2/cc-pVTZ optimized).

| State $n$ | $\lambda_n$ | $E_n$ | $f$   | $-\mathcal{B}$ | Symm. |
|-----------|-------------|-------|-------|----------------|-------|
| 1         | 282.827     | 0.161 | 0.002 | 1.011          | 1A''  |
| 2         | 240.567     | 0.189 | 0.110 | 21.332         | 1A'   |
| 3         | 228.159     | 0.200 | 0.002 | 0.113          | 2A''  |
| 4         | 222.044     | 0.205 | 0.066 | -42.786        | 2A'   |
| 5         | 220.539     | 0.207 | 0.000 | 0.035          | 3A''  |
| 6         | 207.295     | 0.220 | 0.011 | -1.119         | 3A'   |
| 7         | 199.228     | 0.229 | 0.001 | -0.810         | 4A''  |
| 8         | 193.475     | 0.236 | 0.017 | 6.042          | 4A'   |
| 9         | 188.123     | 0.242 | 0.005 | -2.781         | 5A''  |
| 10        | 186.125     | 0.245 | 0.514 | 6.302          | 5A'   |
| 11        | 184.991     | 0.246 | 0.002 | 5.618          | 6A''  |
| 12        | 183.872     | 0.248 | 0.007 | 0.970          | 7A''  |
| 13        | 182.765     | 0.249 | 0.028 | 4.865          | 6A'   |
| 14        | 180.807     | 0.252 | 0.000 | -0.217         | 8A''  |
| 15        | 177.704     | 0.256 | 0.014 | -2.934         | 7A'   |
| 16        | 176.261     | 0.259 | 0.000 | -0.924         | 9A''  |
| 17        | 175.717     | 0.259 | 0.080 | -3.926         | 8A'   |
| 18        | 174.773     | 0.261 | 0.006 | 6.516          | 9A'   |
| 19        | 173.509     | 0.263 | 0.002 | 0.938          | 10A'' |

Table S15: Purine. ADC(2)-x/aug-cc-pVDZ results for excitation wavelengths  $\lambda_n$  (nm), excitation energies  $E_n$  (Hartree), oscillator strengths  $f$  and MCD  $-\mathcal{B}$  terms (atomic units) at planar geometry (MP2/cc-pVTZ optimized).

| State $n$ | $\lambda_n$ | $E_n$ | $f$   | $-\mathcal{B}$ | Symm. |
|-----------|-------------|-------|-------|----------------|-------|
| 1         | 347.547     | 0.131 | 0.002 | 0.991          | 1A''  |
| 2         | 291.886     | 0.156 | 0.067 | 11.825         | 1A'   |
| 3         | 269.287     | 0.169 | 0.002 | 0.412          | 2A''  |
| 4         | 261.708     | 0.174 | 0.000 | -0.134         | 3A''  |
| 5         | 255.830     | 0.178 | 0.062 | -30.724        | 2A'   |
| 6         | 223.240     | 0.204 | 0.010 | 0.191          | 3A'   |
| 7         | 218.634     | 0.208 | 0.006 | -2.656         | 4A''  |
| 8         | 215.940     | 0.211 | 0.000 | -1.980         | 5A''  |
| 9         | 212.913     | 0.214 | 0.416 | 18.806         | 4A'   |

Table S16: Purine. ADC(3)/aug-cc-pVDZ results for excitation wavelengths  $\lambda_n$  (nm), excitation energies  $E_n$  (Hartree), oscillator strengths  $f$  and MCD  $-\mathcal{B}$  terms (atomic units) at planar geometry (MP2/cc-pVTZ optimized).

| State $n$ | $\lambda_n$ | $E_n$ | $f$   | $-\mathcal{B}$ | Symm. |
|-----------|-------------|-------|-------|----------------|-------|
| 1         | 262.916     | 0.173 | 0.003 | 2.200          | 1A''  |
| 2         | 249.936     | 0.182 | 0.114 | 4.726          | 1A'   |
| 3         | 221.828     | 0.205 | 0.061 | -19.823        | 2A'   |
| 4         | 219.160     | 0.208 | 0.002 | 1.847          | 2A''  |
| 5         | 204.595     | 0.223 | 0.000 | 0.011          | 3A''  |
| 6         | 198.793     | 0.229 | 0.001 | -0.733         | 4A''  |
| 7         | 186.659     | 0.244 | 0.400 | -0.317         | 3A'   |
| 8         | 184.392     | 0.247 | 0.009 | 8.477          | 5A''  |
| 9         | 184.243     | 0.247 | 0.021 | -13.180        | 4A'   |
| 10        | 181.455     | 0.251 | 0.000 | -0.048         | 6A''  |
| 11        | 178.890     | 0.255 | 0.002 | 0.130          | 7A''  |
| 12        | 175.988     | 0.259 | 0.005 | 0.802          | 5A'   |

Table S17: Purine. RICC2/aug-cc-pVDZ results for excitation wavelengths  $\lambda_n$  (nm), excitation energies  $E_n$  (Hartree), oscillator strengths  $f$  and MCD  $-\mathcal{B}$  terms (atomic units) at planar geometry (MP2/cc-pVTZ optimized).

| State $n$ | $\lambda_n$ | $E_n$ | $f$   | $-\mathcal{B}$ | Symm. |
|-----------|-------------|-------|-------|----------------|-------|
| 1         | 280.083     | 0.163 | 0.003 | 0.962          | 1A''  |
| 2         | 239.340     | 0.190 | 0.104 | 14.712         | 1A'   |
| 3         | 225.654     | 0.202 | 0.002 | 0.136          | 2A''  |
| 4         | 219.487     | 0.208 | 0.053 | -32.692        | 2A'   |
| 5         | 218.822     | 0.208 | 0.000 | 0.257          | 3A''  |
| 6         | 207.336     | 0.220 | 0.014 | -1.407         | 3A'   |
| 7         | 198.884     | 0.229 | 0.001 | -0.731         | 4A''  |
| 8         | 192.927     | 0.236 | 0.016 | 6.366          | 4A'   |
| 9         | 186.557     | 0.244 | 0.004 | -1.809         | 5A''  |
| 10        | 185.126     | 0.246 | 0.455 | 0.116          | 5A'   |
| 11        | 183.746     | 0.248 | 0.002 | 4.670          | 6A''  |
| 12        | 182.606     | 0.250 | 0.008 | 6.982          | 7A''  |
| 13        | 182.304     | 0.250 | 0.038 | 1.079          | 6A'   |
| 14        | 180.469     | 0.252 | 0.000 | -0.283         | 8A''  |
| 15        | 177.420     | 0.257 | 0.008 | -2.468         | 7A'   |
| 16        | 176.693     | 0.258 | 0.000 | -0.306         | 9A''  |
| 17        | 175.761     | 0.259 | 0.021 | -2.653         | 8A'   |
| 18        | 174.447     | 0.261 | 0.012 | 7.057          | 9A'   |
| 19        | 172.912     | 0.264 | 0.002 | 2.375          | 10A'' |

Table S18: Purine + 4· H<sub>2</sub>O. ADC(2)/aug-cc-pVDZ results for excitation wavelengths  $\lambda_n$  (nm), excitation energies  $E_n$  (Hartree), oscillator strengths  $f$  and MCD  $-\mathcal{B}$  terms (atomic units) at PCM-B3LYP/cc-pVTZ optimized structure, taken from 3.

| State $n$ | $\lambda_n$ | $E_n$ | $-\mathcal{B}$ |
|-----------|-------------|-------|----------------|
| 1         | 274.148     | 0.166 | 0.909          |
| 2         | 238.552     | 0.191 | 34.749         |
| 3         | 224.119     | 0.203 | -59.579        |
| 4         | 223.022     | 0.204 | 0.766          |
| 5         | 216.865     | 0.210 | -0.151         |
| 6         | 197.758     | 0.230 | -1.075         |
| 7         | 190.562     | 0.239 | 0.070          |
| 8         | 187.272     | 0.243 | -3.040         |

Table S19: Hypoxanthine. ADC(2)/aug-cc-pVDZ results for excitation wavelengths  $\lambda_n$  (nm), excitation energies  $E_n$  (Hartree), oscillator strengths  $f$  and MCD  $-\mathcal{B}$  terms (atomic units) at planar geometry (MP2/cc-pVTZ optimized).

| State $n$ | $\lambda_n$ | $E_n$ | $f$   | $-\mathcal{B}$ | Symm. |
|-----------|-------------|-------|-------|----------------|-------|
| 1         | 252.010     | 0.181 | 0.147 | -41.364        | 1A'   |
| 2         | 237.557     | 0.192 | 0.000 | -0.102         | 1A''  |
| 3         | 229.192     | 0.199 | 0.000 | -0.062         | 2A''  |
| 4         | 228.847     | 0.199 | 0.002 | -2.688         | 3A''  |
| 5         | 224.561     | 0.203 | 0.215 | 48.197         | 2A'   |
| 6         | 218.844     | 0.208 | 0.001 | 0.237          | 4A''  |
| 7         | 216.453     | 0.211 | 0.001 | -0.098         | 5A''  |
| 8         | 206.824     | 0.220 | 0.009 | 0.482          | 3A'   |
| 9         | 194.217     | 0.235 | 0.001 | -0.390         | 6A''  |
| 10        | 193.722     | 0.235 | 0.002 | -0.417         | 7A''  |
| 11        | 192.332     | 0.237 | 0.006 | -0.908         | 4A'   |
| 12        | 192.007     | 0.237 | 0.004 | 0.649          | 5A'   |
| 13        | 191.443     | 0.238 | 0.000 | -3.608         | 8A''  |
| 14        | 187.735     | 0.243 | 0.024 | 2.918          | 6A'   |
| 15        | 185.443     | 0.246 | 0.097 | -3.658         | 7A'   |
| 16        | 183.723     | 0.248 | 0.004 | -6.598         | 9A''  |
| 17        | 182.253     | 0.250 | 0.123 | -11.075        | 8A'   |
| 18        | 180.735     | 0.252 | 0.059 | 4.085          | 9A'   |
| 19        | 179.737     | 0.254 | 0.005 | -7.425         | 10A'' |
| 20        | 177.912     | 0.256 | 0.003 | -0.711         | 11A'' |
| 21        | 177.152     | 0.257 | 0.043 | -2.831         | 10A'  |
| 22        | 176.602     | 0.258 | 0.135 | 16.632         | 11A'  |
| 23        | 172.916     | 0.264 | 0.048 | -0.897         | 12A'  |
| 24        | 171.872     | 0.265 | 0.000 | 24.677         | 12A'' |
| 25        | 171.808     | 0.265 | 0.411 | -28.411        | 13A'  |
| 26        | 169.255     | 0.269 | 0.000 | 0.555          | 13A'' |
| 27        | 167.821     | 0.272 | 0.032 | 6.983          | 14A'  |
| 28        | 164.905     | 0.276 | 0.003 | 1.707          | 14A'' |

Table S20: Hypoxanthine. ADC(2)-x/aug-cc-pVDZ results for excitation wavelengths  $\lambda_n$  (nm), excitation energies  $E_n$  (Hartree), oscillator strengths  $f$  and MCD  $-\mathcal{B}$  terms (atomic units) at planar geometry (MP2/cc-pVTZ optimized).

| State $n$ | $\lambda_n$ | $E_n$ | $f$   | $-\mathcal{B}$ | Symm. |
|-----------|-------------|-------|-------|----------------|-------|
| 1         | 301.944     | 0.151 | 0.103 | -31.125        | 1A'   |
| 2         | 273.326     | 0.167 | 0.000 | -0.160         | 1A''  |
| 3         | 264.903     | 0.172 | 0.000 | -0.121         | 2A''  |
| 4         | 260.959     | 0.175 | 0.147 | 31.158         | 2A'   |
| 5         | 256.695     | 0.178 | 0.001 | 0.551          | 3A''  |
| 6         | 249.389     | 0.183 | 0.001 | 0.038          | 4A''  |
| 7         | 234.742     | 0.194 | 0.001 | 0.131          | 5A''  |
| 8         | 224.229     | 0.203 | 0.002 | -3.552         | 3A'   |
| 9         | 221.720     | 0.206 | 0.004 | 1.087          | 6A''  |
| 10        | 221.504     | 0.206 | 0.024 | -1.211         | 4A'   |

Table S21: Hypoxanthine. ADC(3)/aug-cc-pVDZ results for excitation wavelengths  $\lambda_n$  (nm), excitation energies  $E_n$  (Hartree), oscillator strengths  $f$  and MCD  $-\mathcal{B}$  terms (atomic units) at planar geometry (MP2/cc-pVTZ optimized).

| State $n$ | $\lambda_n$ | $E_n$ | $f$   | $-\mathcal{B}$ | Symm. |
|-----------|-------------|-------|-------|----------------|-------|
| 1         | 252.709     | 0.180 | 0.127 | -39.733        | 1A'   |
| 2         | 226.683     | 0.201 | 0.220 | 42.931         | 2A'   |
| 3         | 224.561     | 0.203 | 0.002 | 4.328          | 1A''  |
| 4         | 214.618     | 0.212 | 0.000 | 0.141          | 2A''  |
| 5         | 211.529     | 0.215 | 0.001 | -0.119         | 3A''  |
| 6         | 204.412     | 0.223 | 0.001 | 0.354          | 4A''  |
| 7         | 195.383     | 0.233 | 0.019 | -1.214         | 3A'   |
| 8         | 192.007     | 0.237 | 0.001 | 0.705          | 5A''  |
| 9         | 188.045     | 0.242 | 0.003 | -0.688         | 6A''  |
| 10        | 187.890     | 0.243 | 0.004 | 1.709          | 7A''  |
| 11        | 184.094     | 0.248 | 0.006 | 0.092          | 4A'   |
| 12        | 180.164     | 0.253 | 0.006 | -2.346         | 8A''  |
| 13        | 178.470     | 0.255 | 0.341 | -22.425        | 5A'   |

Table S22: Hypoxanthine. RICC2/aug-cc-pVDZ results for excitation wavelengths  $\lambda_n$  (nm), excitation energies  $E_n$  (Hartree), oscillator strengths  $f$  and MCD  $-\mathcal{B}$  terms (atomic units) at planar geometry (MP2/cc-pVTZ optimized).

| State $n$ | $\lambda_n$ | $E_n$ | $f$   | $-\mathcal{B}$ | Symm. |
|-----------|-------------|-------|-------|----------------|-------|
| 1         | 245.534     | 0.186 | 0.140 | -40.749        | 1A'   |
| 2         | 227.746     | 0.200 | 0.002 | -1.539         | 1A''  |
| 3         | 227.152     | 0.201 | 0.000 | -0.564         | 2A''  |
| 4         | 221.955     | 0.205 | 0.197 | 43.922         | 2A'   |
| 5         | 221.657     | 0.206 | 0.000 | 4.475          | 3A''  |
| 6         | 215.711     | 0.211 | 0.001 | 0.116          | 4A''  |
| 7         | 215.282     | 0.212 | 0.000 | -0.155         | 5A''  |
| 8         | 201.987     | 0.226 | 0.013 | 0.202          | 3A'   |
| 9         | 193.397     | 0.236 | 0.001 | -0.597         | 6A''  |
| 10        | 192.748     | 0.236 | 0.002 | -0.589         | 7A''  |
| 11        | 191.971     | 0.237 | 0.003 | -0.626         | 4A'   |
| 12        | 191.605     | 0.238 | 0.009 | 1.225          | 5A'   |
| 13        | 190.682     | 0.239 | 0.001 | -2.295         | 8A''  |
| 14        | 185.362     | 0.246 | 0.023 | 1.565          | 6A'   |
| 15        | 183.758     | 0.248 | 0.024 | -1.203         | 7A'   |
| 16        | 182.923     | 0.249 | 0.005 | -5.816         | 9A''  |
| 17        | 181.240     | 0.251 | 0.011 | -6.171         | 8A'   |
| 18        | 179.823     | 0.253 | 0.127 | -20.617        | 9A'   |
| 19        | 177.481     | 0.257 | 0.002 | -1.967         | 10A'' |
| 20        | 177.127     | 0.257 | 0.007 | -2.901         | 11A'' |
| 21        | 174.373     | 0.261 | 0.189 | 27.794         | 10A'  |
| 22        | 173.361     | 0.263 | 0.073 | 16.709         | 11A'  |
| 23        | 170.855     | 0.267 | 0.290 | -23.136        | 12A'  |

Table S23: Hypoxanthine + 5 water molecules. ADC(2)/aug-cc-pVDZ results for excitation wavelengths  $\lambda_n$  (nm), excitation energies  $E_n$  (Hartree), oscillator strengths  $f$  and MCD  $-\mathcal{B}$  terms (atomic units) at PCM-B3LYP/cc-pVTZ optimized structure, taken from 3.

| State $n$ | $\lambda_n$ | $E_n$ | $-\mathcal{B}$ |
|-----------|-------------|-------|----------------|
| 1         | 249.936     | 0.182 | -66.710        |
| 2         | 231.802     | 0.197 | 72.246         |
| 3         | 231.005     | 0.197 | 5.294          |
| 4         | 221.477     | 0.206 | -0.067         |
| 5         | 214.187     | 0.213 | 0.185          |
| 6         | 212.714     | 0.214 | 0.331          |
| 7         | 198.793     | 0.229 | 0.019          |

### 1.3. 1,4-naphthoquinone

Table S24: 1,4-naphthoquinone. ADC(2)/aug-cc-pVDZ results for excitation wavelengths  $\lambda_n$  (nm), excitation energies  $E_n$  (Hartree), oscillator strengths  $f$  and MCD  $-\mathcal{B}$  terms (atomic units) at planar geometry (B3LYP/cc-pVTZ optimized).

| State $n$ | $\lambda_n$ | $E_n$ | $f$   | $-\mathcal{B}$ | Symm. |
|-----------|-------------|-------|-------|----------------|-------|
| 1         | 435.180     | 0.105 | 0.000 | -0.023         | 1B2   |
| 2         | 297.605     | 0.153 | 0.053 | 26.940         | 1A1   |
| 3         | 283.354     | 0.161 | 0.047 | -26.355        | 1B1   |
| 4         | 236.447     | 0.193 | 0.000 | -0.044         | 2B2   |
| 5         | 228.847     | 0.199 | 0.401 | 6.347          | 2B1   |
| 6         | 224.671     | 0.203 | 0.161 | 12.572         | 2A1   |
| 7         | 220.860     | 0.206 | 0.000 | 0.613          | 3B2   |
| 8         | 203.954     | 0.223 | 0.065 | -51.131        | 3B1   |
| 9         | 199.489     | 0.228 | 0.006 | 1.825          | 4B1   |
| 10        | 194.300     | 0.235 | 0.025 | -0.757         | 3A1   |
| 11        | 184.243     | 0.247 | 0.011 | -0.334         | 5B1   |
| 12        | 184.094     | 0.248 | 0.396 | -63.605        | 4A1   |
| 13        | 183.427     | 0.248 | 0.001 | 1.719          | 4B2   |
| 14        | 179.666     | 0.254 | 0.190 | 146.847        | 6B1   |
| 15        | 179.031     | 0.255 | 0.020 | 0.806          | 5A1   |
| 16        | 178.680     | 0.255 | 0.012 | 13.576         | 5B2   |
| 17        | 177.220     | 0.257 | 0.322 | -89.315        | 6A1   |

Table S25: 1,4-naphthoquinone. RICC2/aug-cc-pVDZ results for excitation wavelengths  $\lambda_n$  (nm), excitation energies  $E_n$  (Hartree), oscillator strengths  $f$  and MCD  $-\mathcal{B}$  terms (atomic units) at planar geometry (B3LYP/cc-pVTZ optimized).

| State $n$ | $\lambda_n$ | $E_n$ | $f$   | $-\mathcal{B}$ | Symm. |
|-----------|-------------|-------|-------|----------------|-------|
| 1         | 414.566     | 0.110 | 0.000 | -0.027         | 1B2   |
| 2         | 299.418     | 0.152 | 0.048 | 24.754         | 1A1   |
| 3         | 287.525     | 0.158 | 0.029 | -23.533        | 1B1   |
| 4         | 232.029     | 0.196 | 0.000 | -0.076         | 2B2   |
| 5         | 224.747     | 0.203 | 0.156 | 28025.426      | 2A1   |
| 6         | 224.745     | 0.203 | 0.354 | 28001.101      | 2B1   |
| 7         | 218.271     | 0.209 | 0.000 | 0.511          | 3B2   |
| 8         | 203.588     | 0.224 | 0.056 | -46.412        | 3B1   |
| 9         | 198.106     | 0.230 | 0.007 | 2.032          | 4B1   |
| 10        | 191.907     | 0.237 | 0.026 | -0.343         | 3A1   |
| 11        | 184.469     | 0.247 | 0.001 | -0.422         | 4B2   |
| 12        | 183.575     | 0.248 | 0.016 | -1.900         | 5B1   |
| 13        | 183.275     | 0.249 | 0.451 | -62.422        | 4A1   |
| 14        | 179.746     | 0.253 | 0.011 | -15.915        | 5B2   |
| 15        | 179.056     | 0.254 | 0.175 | 194.654        | 6B1   |
| 16        | 177.741     | 0.256 | 0.100 | -46.250        | 5A1   |
| 17        | 177.355     | 0.257 | 0.227 | -60.947        | 6A1   |
| 18        | 175.752     | 0.259 | 0.036 | -72.070        | 7A1   |
| 19        | 175.728     | 0.259 | 0.024 | 45.361         | 7B1   |
| 20        | 173.185     | 0.263 | 0.021 | 11.398         | 8B1   |
| 21        | 170.938     | 0.267 | 0.003 | -1.808         | 9B1   |
| 22        | 166.931     | 0.273 | 0.004 | -2.669         | 8A1   |
| 23        | 166.552     | 0.274 | 0.000 | -5.074         | 6B2   |
| 24        | 166.548     | 0.274 | 0.022 | -30.255        | 9A1   |
| 25        | 166.327     | 0.274 | 0.014 | 29.085         | 7B2   |
| 26        | 164.997     | 0.276 | 0.013 | 0.811          | 8B2   |
| 27        | 162.433     | 0.281 | 0.009 | 8.010          | 10B1  |

## 1.4. 9,10-anthraquinone

Table S26: 9,10-anthraquinone. ADC(2)/aug-cc-pVDZ results for excitation wavelengths  $\lambda_n$  (nm), excitation energies  $E_n$  (Hartree), oscillator strengths  $f$  and MCD  $-\mathcal{B}$  terms (atomic units) at planar geometry (B3LYP/cc-pVTZ optimized).

| State $n$ | $\lambda_n$ | $E_n$ | $f$   | $-\mathcal{B}$ | Symm.             |
|-----------|-------------|-------|-------|----------------|-------------------|
| 1         | 284.416     | 0.160 | 0.080 | 18.400         | 1B <sub>3u</sub>  |
| 2         | 246.023     | 0.185 | 0.300 | -15.465        | 1B <sub>2u</sub>  |
| 3         | 225.897     | 0.202 | 0.761 | 196.208        | 2B <sub>3u</sub>  |
| 4         | 220.539     | 0.207 | 0.000 | -0.985         | 1B <sub>1u</sub>  |
| 5         | 217.798     | 0.209 | 0.129 | -278.555       | 2B <sub>2u</sub>  |
| 6         | 198.102     | 0.230 | 0.031 | -1.603         | 3B <sub>3u</sub>  |
| 7         | 194.052     | 0.235 | 0.001 | 0.349          | 2B <sub>1u</sub>  |
| 8         | 189.531     | 0.240 | 0.000 | -2.295         | 3B <sub>2u</sub>  |
| 9         | 188.590     | 0.242 | 0.802 | -2.104         | 4B <sub>3u</sub>  |
| 10        | 182.985     | 0.249 | 0.017 | -1.230         | 5B <sub>3u</sub>  |
| 11        | 179.879     | 0.253 | 0.031 | 0.940          | 4B <sub>2u</sub>  |
| 12        | 179.525     | 0.254 | 0.020 | 5.594          | 3B <sub>1u</sub>  |
| 13        | 175.717     | 0.259 | 0.146 | 6.075          | 5B <sub>2u</sub>  |
| 14        | 173.575     | 0.263 | 0.012 | -2.530         | 6B <sub>3u</sub>  |
| 15        | 169.949     | 0.268 | 0.003 | 7.476          | 6B <sub>2u</sub>  |
| 16        | 168.504     | 0.270 | 0.269 | 95.700         | 7B <sub>3u</sub>  |
| 17        | 168.007     | 0.271 | 0.041 | 31.681         | 4B <sub>1u</sub>  |
| 18        | 166.108     | 0.274 | 0.000 | 0.254          | 5B <sub>1u</sub>  |
| 19        | 165.745     | 0.275 | 0.007 | 10.894         | 6B <sub>1u</sub>  |
| 20        | 164.429     | 0.277 | 0.019 | -7569.812      | 8B <sub>3u</sub>  |
| 21        | 164.429     | 0.277 | 0.666 | 7663.730       | 7B <sub>2u</sub>  |
| 22        | 164.192     | 0.278 | 0.023 | -170.643       | 8B <sub>2u</sub>  |
| 23        | 160.434     | 0.284 | 0.005 | 0.256          | 9B <sub>3u</sub>  |
| 24        | 159.759     | 0.285 | 0.000 | -0.040         | 7B <sub>1u</sub>  |
| 25        | 157.604     | 0.289 | 0.004 | 0.858          | 9B <sub>2u</sub>  |
| 26        | 155.030     | 0.294 | 0.002 | 0.480          | 8B <sub>1u</sub>  |
| 27        | 154.819     | 0.294 | 0.005 | 3.754          | 10B <sub>2u</sub> |

Table S27: 9,10-anthraquinone. RICC2/aug-cc-pVDZ results for excitation wavelengths  $\lambda_n$  (nm), excitation energies  $E_n$  (Hartree), oscillator strengths  $f$  and MCD  $-\mathcal{B}$  terms (atomic units) at planar geometry (B3LYP/cc-pVTZ optimized).

| State $n$ | $\lambda_n$ | $E_n$ | $f$    | $-\mathcal{B}$ | Symm.             |
|-----------|-------------|-------|--------|----------------|-------------------|
| 1         | 286.385     | 0.159 | 0.073  | 13.297         | 1B <sub>3u</sub>  |
| 2         | 242.401     | 0.188 | 0.254  | -4.041         | 1B <sub>2u</sub>  |
| 3         | 227.157     | 0.201 | 0.744  | 135.146        | 2B <sub>3u</sub>  |
| 4         | 218.052     | 0.209 | 0.000  | -0.764         | 1B <sub>1u</sub>  |
| 5         | 217.390     | 0.210 | 0.105  | -219.913       | 2B <sub>2u</sub>  |
| 6         | 195.325     | 0.233 | 0.030  | -1.078         | 3B <sub>3u</sub>  |
| 7         | 191.206     | 0.238 | 0.001  | 1.989          | 2B <sub>1u</sub>  |
| 8         | 188.805     | 0.241 | 0.001  | -18.363        | 3B <sub>2u</sub>  |
| 9         | 188.602     | 0.242 | 0.785  | 11.661         | 4B <sub>3u</sub>  |
| 10        | 182.680     | 0.249 | 0.014  | -1.325         | 5B <sub>3u</sub>  |
| 11        | 180.152     | 0.253 | 0.020  | -14.711        | 3B <sub>1u</sub>  |
| 12        | 179.786     | 0.253 | 0.057  | 27.724         | 4B <sub>2u</sub>  |
| 13        | 175.169     | 0.260 | 0.108  | -2.203         | 5B <sub>2u</sub>  |
| 14        | 171.710     | 0.265 | 0.015  | -6.936         | 6B <sub>3u</sub>  |
| 15        | 168.867     | 0.270 | 0.002  | 6.638          | 6B <sub>2u</sub>  |
| 16        | 168.406     | 0.271 | 0.043  | -7.156         | 4B <sub>1u</sub>  |
| 17        | 167.883     | 0.271 | 0.269  | 175.003        | 7B <sub>3u</sub>  |
| 18        | 166.599     | 0.273 | 0.001  | 1.772          | 5B <sub>1u</sub>  |
| 19        | 166.402     | 0.274 | 0.002  | 5.125          | 6B <sub>1u</sub>  |
| 20        | 165.009     | 0.276 | 0.629  | -126.922       | 7B <sub>2u</sub>  |
| 21        | 163.762     | 0.278 | -0.000 | 0.107          | 8B <sub>2u</sub>  |
| 22        | 163.525     | 0.279 | 0.018  | -13.477        | 8B <sub>3u</sub>  |
| 23        | 160.835     | 0.283 | 0.000  | -0.015         | 7B <sub>1u</sub>  |
| 24        | 159.703     | 0.285 | 0.012  | -1.548         | 9B <sub>3u</sub>  |
| 25        | 157.119     | 0.290 | 0.003  | 0.620          | 9B <sub>2u</sub>  |
| 26        | 155.545     | 0.293 | 0.002  | -0.661         | 8B <sub>1u</sub>  |
| 27        | 155.186     | 0.294 | 0.002  | 35.369         | 10B <sub>2u</sub> |

## 1.5. 1-Naphthylamine

Table S28: 1-Naphthylamine. RICC2/aug-cc-pVDZ results for excitation wavelengths  $\lambda_n$  (nm), excitation energies  $E_n$  (Hartree), oscillator strengths  $f$  and MCD  $-B$  terms (atomic units) at planar geometry (CC2/aug-cc-pVDZ optimized).

| State $n$ | $\lambda_n$ | $E_n$ | $f$   | $-B$     | Symm. |
|-----------|-------------|-------|-------|----------|-------|
| 1         | 310.877     | 0.147 | 0.109 | -172.901 | 1A'   |
| 2         | 302.156     | 0.151 | 0.044 | 176.685  | 2A'   |
| 3         | 291.318     | 0.156 | 0.008 | -0.845   | 1A''  |
| 4         | 259.137     | 0.176 | 0.001 | 0.058    | 2A''  |
| 5         | 253.336     | 0.180 | 0.001 | 0.052    | 3A''  |
| 6         | 232.684     | 0.196 | 0.379 | -27.029  | 3A'   |
| 7         | 230.673     | 0.198 | 0.003 | -4.347   | 4A''  |
| 8         | 229.901     | 0.198 | 0.003 | -4.776   | 5A''  |
| 9         | 221.935     | 0.205 | 0.086 | 16.610   | 4A'   |
| 10        | 218.211     | 0.209 | 0.001 | -1.595   | 6A''  |
| 11        | 213.988     | 0.213 | 0.004 | 8.099    | 5A'   |
| 12        | 207.194     | 0.220 | 0.013 | -23.532  | 7A''  |
| 13        | 207.154     | 0.220 | 0.019 | 17.837   | 6A'   |
| 14        | 206.346     | 0.221 | 0.000 | -0.712   | 8A''  |
| 15        | 203.793     | 0.224 | 0.002 | 0.280    | 9A''  |
| 16        | 198.616     | 0.229 | 0.766 | -187.625 | 7A'   |
| 17        | 198.051     | 0.230 | 0.000 | -0.267   | 10A'' |

Table S29: 1-Naphthylamine. ADC(2)/aug-cc-pVDZ results for excitation wavelengths  $\lambda_n$  (nm), excitation energies  $E_n$  (Hartree), oscillator strengths  $f$  and MCD  $-B$  terms (atomic units) at planar geometry (CC2/aug-cc-pVDZ optimized).

| State $n$ | $\lambda_n$ | $E_n$ | $f$   | $-B$     | Symm. |
|-----------|-------------|-------|-------|----------|-------|
| 1         | 312.935     | 0.146 | 0.122 | -170.089 | 1A'   |
| 2         | 302.747     | 0.151 | 0.050 | 175.398  | 2A'   |
| 3         | 290.583     | 0.157 | 0.007 | -0.849   | 1A''  |
| 4         | 258.883     | 0.176 | 0.001 | 0.055    | 2A''  |
| 5         | 252.849     | 0.180 | 0.001 | 0.088    | 3A''  |
| 6         | 233.299     | 0.195 | 0.405 | -34.477  | 3A'   |
| 7         | 230.351     | 0.198 | 0.003 | -4.129   | 4A''  |
| 8         | 229.538     | 0.199 | 0.003 | -4.253   | 5A''  |
| 9         | 222.913     | 0.204 | 0.088 | 25.579   | 4A'   |
| 10        | 217.798     | 0.209 | 0.001 | -0.937   | 6A''  |
| 11        | 214.315     | 0.213 | 0.003 | 4.928    | 5A'   |
| 12        | 206.918     | 0.220 | 0.017 | -10.104  | 6A'   |
| 13        | 206.730     | 0.220 | 0.011 | 4.710    | 7A''  |
| 14        | 205.518     | 0.222 | 0.003 | -2.511   | 8A''  |
| 15        | 203.590     | 0.224 | 0.002 | 0.047    | 9A''  |
| 16        | 198.620     | 0.229 | 0.806 | -210.648 | 7A'   |
| 17        | 197.329     | 0.231 | 0.000 | -0.061   | 10A'' |

## 2. GEOMETRIES

Table S30: Structure of uracil (Å). Optimised at MP2/cc-pVTZ level of theory in gas-phase.

| Atom | X         | Y         | Z        |
|------|-----------|-----------|----------|
| N    | 0.034463  | -0.977399 | 0.000000 |
| N    | -1.172878 | 0.982298  | 0.000000 |
| C    | -0.007142 | 1.702137  | 0.000000 |
| C    | -1.219536 | -0.402117 | 0.000000 |
| C    | 1.287978  | -0.346449 | 0.000000 |
| C    | 1.201070  | 1.104334  | 0.000000 |
| O    | -2.259216 | -1.030438 | 0.000000 |
| O    | 2.312737  | -1.005372 | 0.000000 |
| H    | -2.068828 | 1.440224  | 0.000000 |
| H    | -0.123380 | 2.775675  | 0.000000 |
| H    | 0.046519  | -1.988139 | 0.000000 |
| H    | 2.112201  | 1.676991  | 0.000000 |

Table S31: Structure of uracil surrounded by 4 water molecules (Å). Optimised at PCM/B3LYP/cc-pVTZ level of theory, taken from Ref. 3.

| Atom | X         | Y         | Z         |
|------|-----------|-----------|-----------|
| N    | -0.244586 | -0.305278 | 0.164159  |
| N    | 1.989498  | -0.868165 | -0.053061 |
| C    | 1.057160  | 0.122713  | 0.121078  |
| C    | 1.653590  | -2.183393 | -0.179396 |
| C    | 0.369678  | -2.593401 | -0.146976 |
| C    | -0.679845 | -1.621943 | 0.026537  |
| O    | 1.375244  | 1.308342  | 0.231897  |
| O    | -1.882880 | -1.889431 | 0.060695  |
| O    | -2.331488 | 1.698854  | 0.574128  |
| O    | 4.193760  | 0.952935  | -0.023860 |
| O    | -0.424573 | 3.439829  | -0.665405 |
| O    | -4.064961 | -0.228061 | -0.193037 |
| H    | -0.956698 | 0.418717  | 0.323520  |
| H    | 2.960886  | -0.552990 | -0.081033 |
| H    | 2.481760  | -2.863587 | -0.308683 |
| H    | 0.104642  | -3.631740 | -0.251583 |
| H    | 0.276149  | 2.830350  | -0.390313 |
| H    | -3.335009 | -0.879789 | -0.125244 |
| H    | -3.082062 | 1.128118  | 0.284358  |
| H    | -2.498930 | 1.912585  | 1.497877  |
| H    | -1.223122 | 3.000050  | -0.336334 |
| H    | 3.362976  | 1.436278  | 0.123472  |
| H    | 4.672663  | 1.015813  | 0.809368  |
| H    | -4.301946 | -0.203296 | -1.125888 |

Table S32: Structure of 2-thiouracil (bohr), optimised at RI-MP2/cc-pVTZ level of theory in gas-phase.

| Atom | X         | Y         | Z        |
|------|-----------|-----------|----------|
| S    | 4.633388  | 0.848464  | 0.000000 |
| O    | -4.459288 | 2.805377  | 0.000000 |
| N    | 0.910404  | -2.484051 | 0.000000 |
| N    | -0.329419 | 1.635591  | 0.000000 |
| C    | 1.648769  | -0.009686 | 0.000000 |
| C    | -2.924040 | 1.099513  | 0.000000 |
| C    | -3.465011 | -1.575008 | 0.000000 |
| C    | -1.551570 | -3.245522 | 0.000000 |
| H    | 2.331760  | -3.745504 | 0.000000 |
| H    | 0.136210  | 3.486215  | 0.000000 |
| H    | -5.397002 | -2.179171 | 0.000000 |
| H    | -1.846647 | -5.256529 | 0.000000 |

Table S33: Structure of 4-thiouracil ( $\text{\AA}$ ), optimised at B3LYP/cc-pVTZ level of theory in gas-phase.

| Atom | X         | Y         | Z        |
|------|-----------|-----------|----------|
| N    | -0.113158 | -0.863056 | 0.000000 |
| N    | -1.788377 | 0.731593  | 0.000000 |
| C    | -1.476675 | -0.621577 | 0.000000 |
| C    | -0.840516 | 1.720924  | 0.000000 |
| C    | 0.476661  | 1.434134  | 0.000000 |
| C    | 0.916628  | 0.064689  | 0.000000 |
| O    | -2.315390 | -1.493374 | 0.000000 |
| S    | 2.499895  | -0.423509 | 0.000000 |
| H    | -2.772031 | 0.946304  | 0.000000 |
| H    | -1.218715 | 2.733106  | 0.000000 |
| H    | 1.218865  | 2.213753  | 0.000000 |
| H    | 0.150838  | -1.838814 | 0.000000 |

Table S34: Structure of purine ( $\text{\AA}$ ), optimised at MP2/cc-pVTZ level of theory in gas-phase.

| Atom | X         | Y         | Y        |
|------|-----------|-----------|----------|
| N    | -0.884921 | -1.427211 | 0.000000 |
| N    | -2.112628 | 0.653794  | 0.000000 |
| N    | 1.521196  | -1.056040 | 0.000000 |
| N    | 1.545129  | 1.200398  | 0.000000 |
| C    | 0.206152  | -0.667991 | 0.000000 |
| C    | 0.245874  | 0.739070  | 0.000000 |
| C    | -0.992558 | 1.378469  | 0.000000 |
| C    | -2.001412 | -0.690397 | 0.000000 |
| C    | 2.264210  | 0.094791  | 0.000000 |
| H    | 1.862181  | -2.003010 | 0.000000 |
| H    | 3.341555  | 0.065538  | 0.000000 |
| H    | -2.932531 | -1.240033 | 0.000000 |
| H    | -1.086234 | 2.457257  | 0.000000 |

Table S35: Structure of hypoxanthine (Å), optimised at MP2/cc-pVTZ level of theory in gas-phase.

| Atom | X         | Y         | Z        |
|------|-----------|-----------|----------|
| N    | -1.321641 | -1.414613 | 0.000000 |
| N    | -2.000283 | 0.723668  | 0.000000 |
| N    | 1.903461  | 0.329365  | 0.000000 |
| N    | 0.130649  | 1.887434  | 0.000000 |
| C    | -0.238629 | -0.575189 | 0.000000 |
| C    | -0.634162 | 0.762403  | 0.000000 |
| C    | -2.359202 | -0.595628 | 0.000000 |
| C    | 1.168858  | -0.889339 | 0.000000 |
| C    | 1.399981  | 1.594512  | 0.000000 |
| H    | -2.608816 | 1.525805  | 0.000000 |
| H    | -3.391007 | -0.903446 | 0.000000 |
| H    | 2.130460  | 2.392096  | 0.000000 |
| H    | 2.906902  | 0.205642  | 0.000000 |
| O    | 1.744509  | -1.960205 | 0.000000 |

Table S36: Structure of purine surrounded by 4 water molecules (Å), optimised at PCM/B3LYP/cc-pVTZ level of theory, taken from Ref. 3.

| Atom | X         | Y         | Z         |
|------|-----------|-----------|-----------|
| C    | -0.541878 | 0.041310  | 0.004631  |
| C    | 0.699604  | 0.707806  | 0.017053  |
| C    | 1.829903  | -0.090036 | -0.003752 |
| C    | 0.459571  | -1.943224 | -0.043580 |
| C    | -0.805885 | 2.211080  | 0.056315  |
| H    | 2.832719  | 0.318257  | 0.003700  |
| H    | 0.396426  | -3.023089 | -0.067899 |
| H    | -2.504589 | 0.908805  | 0.030303  |
| H    | -1.325965 | 3.154512  | 0.079702  |
| H    | -4.797291 | 0.804844  | 0.802632  |
| H    | -4.802468 | 0.850937  | -0.731103 |
| H    | -2.544658 | -2.095953 | -0.046958 |
| H    | -3.932982 | -1.475456 | -0.033301 |
| H    | 3.147993  | 3.657294  | -0.917254 |
| H    | 2.051361  | 3.186566  | 0.040815  |
| H    | 4.334152  | -3.017668 | 0.906438  |
| H    | 3.272989  | -2.464574 | -0.049500 |
| N    | 0.497603  | 2.073745  | 0.050068  |
| N    | -1.486782 | 1.026335  | 0.030171  |
| N    | -0.694520 | -1.278303 | -0.025173 |
| N    | 1.692611  | -1.418947 | -0.035296 |
| O    | -4.309175 | 0.511043  | 0.024584  |
| O    | -3.487315 | -2.333440 | -0.055247 |
| O    | 2.921963  | 3.629669  | 0.017450  |
| O    | 4.119783  | -2.955510 | -0.029283 |

Table S37: Structure of hypoxanthine surrounded by 5 water molecules ( $\text{\AA}$ ), optimised at the PCM/B3LYP/cc-pVTZ level of theory, taken from Ref. 3.

| Atom | X         | Y         | Z         |
|------|-----------|-----------|-----------|
| N    | 1.324444  | -1.210870 | 0.034584  |
| N    | -1.030393 | -1.197200 | 0.018674  |
| N    | 0.318896  | 2.225067  | -0.012008 |
| N    | 2.222589  | 1.053395  | 0.015776  |
| C    | 1.212774  | 0.140819  | 0.019402  |
| C    | 0.031489  | 0.877683  | 0.001946  |
| C    | -1.218914 | 0.187950  | 0.000663  |
| C    | 0.171280  | -1.818553 | 0.033419  |
| C    | 1.630325  | 2.282802  | -0.002798 |
| O    | -2.247672 | 3.616236  | -0.044761 |
| O    | -4.812198 | -0.600149 | -0.126568 |
| O    | 3.943423  | -2.343414 | -0.094807 |
| O    | -2.358642 | 0.675108  | -0.017348 |
| O    | -3.302977 | -2.874136 | -0.007505 |
| O    | 4.897394  | 0.222157  | 0.038378  |
| H    | 2.210878  | 3.189951  | -0.008733 |
| H    | -1.292209 | 3.435420  | -0.036969 |
| H    | -2.595734 | 2.713088  | -0.038737 |
| H    | -5.270952 | -0.410421 | 0.698425  |
| H    | -3.980753 | -0.082869 | -0.084573 |
| H    | 3.003499  | -2.061999 | -0.042288 |
| H    | 4.042404  | -2.734172 | -0.969350 |
| H    | -1.874007 | -1.798080 | 0.024844  |
| H    | -3.990832 | -2.171213 | -0.030908 |
| H    | -3.417347 | -3.316962 | 0.839855  |
| H    | 3.235184  | 0.843577  | 0.034107  |
| H    | 5.324784  | 0.350090  | 0.891612  |
| H    | 4.701042  | -0.740743 | -0.015669 |
| H    | 0.138949  | -2.899037 | 0.044309  |

Table S38: Structure of 1,4-naphthoquinone (bohr), optimised at B3LYP/cc-pVTZ level of theory.

| Atom | X         | Y        | Z         |
|------|-----------|----------|-----------|
| C    | -1.322187 | 0.000000 | 4.658918  |
| C    | -2.646081 | 0.000000 | 2.382180  |
| C    | -1.331138 | 0.000000 | 0.090490  |
| C    | 1.331138  | 0.000000 | 0.090490  |
| C    | 2.646081  | 0.000000 | 2.382180  |
| C    | 1.322187  | 0.000000 | 4.658918  |
| H    | -2.347750 | 0.000000 | 6.437530  |
| H    | -4.696393 | 0.000000 | 2.334258  |
| C    | -2.764229 | 0.000000 | -2.337449 |
| C    | 2.764229  | 0.000000 | -2.337449 |
| H    | 4.696393  | 0.000000 | 2.334258  |
| H    | 2.347750  | 0.000000 | 6.437530  |
| C    | 1.269527  | 0.000000 | -4.712585 |
| C    | -1.269527 | 0.000000 | -4.712585 |
| H    | 2.369252  | 0.000000 | -6.446700 |
| H    | -2.369252 | 0.000000 | -6.446700 |
| O    | 5.079395  | 0.000000 | -2.406641 |
| O    | -5.079395 | 0.000000 | -2.406641 |

Table S39: Structure of 9,10-anthraquinone (Å), optimised at B3LYP/cc-pVTZ level of theory.

| Atom | X         | Y         | Z        |
|------|-----------|-----------|----------|
| O    | 0.000000  | -2.692784 | 0.000000 |
| O    | 0.000000  | 2.692784  | 0.000000 |
| C    | -1.272934 | 0.701204  | 0.000000 |
| C    | -1.272934 | -0.701204 | 0.000000 |
| C    | 1.272934  | 0.701204  | 0.000000 |
| C    | 1.272934  | -0.701204 | 0.000000 |
| C    | 0.000000  | -1.474480 | 0.000000 |
| C    | 0.000000  | 1.474480  | 0.000000 |
| C    | -2.484616 | 1.391714  | 0.000000 |
| C    | -2.484616 | -1.391714 | 0.000000 |
| C    | 2.484616  | 1.391714  | 0.000000 |
| C    | 2.484616  | -1.391714 | 0.000000 |
| C    | -3.683655 | -0.696993 | 0.000000 |
| C    | 3.683655  | -0.696993 | 0.000000 |
| C    | 3.683655  | 0.696993  | 0.000000 |
| C    | -3.683655 | 0.696993  | 0.000000 |
| H    | -2.460476 | 2.472047  | 0.000000 |
| H    | -2.460476 | -2.472047 | 0.000000 |
| H    | 2.460476  | 2.472047  | 0.000000 |
| H    | 2.460476  | -2.472047 | 0.000000 |
| H    | -4.620356 | -1.238047 | 0.000000 |
| H    | 4.620356  | -1.238047 | 0.000000 |
| H    | 4.620356  | 1.238047  | 0.000000 |
| H    | -4.620356 | 1.238047  | 0.000000 |

## REFERENCES

- <sup>1</sup>Wolfgang Voelter, Ruth Records, Edward Bunnenberg, and Carl Djerassi. Magnetic circular dichroism studies. VI. Investigation of some purines, pyrimidines, and nucleosides. J. Am. Chem. Soc., 90(22):6163–6170, 1968.
- <sup>2</sup>Nobuko Igarashi-Yamamoto, Akio Tajiri, Masahiro Hatano, Susumu Shibuya, and Tohru Ueda. Ultraviolet absorption, circular dichroism and magnetic circular dichroism studies of sulfur-containing nucleic acid bases and their nucleosides. BBA - Nucleic Acids and Protein Synthesis, 656(1):1–15, 1981.
- <sup>3</sup>Tobias Fahleson, Joanna Kauczor, Patrick Norman, Fabrizio Santoro, Roberto Improta, and Sonia Coriani. TD-DFT Investigation of the Magnetic Circular Dichroism Spectra of Some Purine and Pyrimidine Bases of Nucleic Acids. J. Phys. Chem. A, 119(21):5476–5489, 2015.
- <sup>4</sup>Carl Djerassi, Edward Bunnenberg, and Danny L. Elder. Organic chemical applications of magnetic circular dichroism. Pure Appl. Chem., 25(1):57–90, 1971.
- <sup>5</sup>John Clark Sutherland and Kathleen Griffin. Magnetic circular dichroism of adenine, hypoxanthine, and guanosine 5'-diphosphate to 180 nm. Biopolymers: Original Research on Biomolecules, 23(12):2715–2724, 1984.
